# Supplementary material for: Non-Gaussian displacements in active transport on a carpet of motile cells
Source: arXiv:2311.05377 source file (2023-11-09)
Supplement: Supplementary file 1 [file SM.pdf]

# SUPPLEMENTAL MATERIAL

## Non-Gaussian displacements in active transport on a carpet of motile cells

Robert Großman, Lara S. Bort, Ted Moldenhawer, Setareh Sharifi Panah, Ralf Metzler, and Carsten Beta

### DESCRIPTION OF MOVIES

Movie 1 shows an exemplary experimental recording of polystyrene particles with a diameter of 46 µm whose motion is driven by a monolayer of *D. discoideum* cells over four hours. The frames in this movie were corrected for spurious motion of the microscope stage (see Material and Methods below for details). The recorded trajectories are shown as an overlay in color.

### MATERIAL AND METHODS

*Cell culturing.* AX2-214 wild-type *D. discoideum* cells were cultivated in untreated polystyrene cell culture flasks (T-75 Standard, Sarstedt AG & Co. KG, Nümbrecht, Germany) in HL5 medium including glucose (Formedium Ltd. Norfolk, England), supplemented with 100 units/ml Penicillin G sodium salt and 0.1 mg/ml Streptomycin sulfate (Penicillin-Streptomycin 10X Solution, Biological Industries, Beit Haemek, Israel) at 20 °C. The culture medium was changed every two to three days. The cells were diluted regularly in order to avoid confluency. The cell culture was renewed once every four weeks at the latest.

*Sample preparation.* After the cells had been harvested, the cell density was adjusted to $1 \cdot 10^6\,\mathrm{ml}^{-1}$ in fresh nutrient medium. The experiment was performed using a 'µ-Slide 8 Well high Grid-500' (ibidi GmbH, Martinsried, Germany). Each well of the µ-slide was filled with 298 µl of the cell solution, leading to a density of approximately $3 \cdot 10^5$ cells per well. After 20 minutes, the cells settled and adhered to the bottom.

Monodispersed spherical polystyrene particles (microParticles GmbH, Berlin, Germany) with a diameter of $(46.30 \pm 0.37)$ µm were diluted in deionized water to a density of $0.3{\cdot}10^3\,\mu\mathrm{l}^{-1}$. After the cells had adhered, 2 µl of the homogeneous particle solution were pipetted just below the surface of the nutrient medium into the well. Afterwards, the µ-slide was slightly tilted to distribute particles most evenly. Particles sedimented for 20 to 55 minutes prior to the experiment.

*Imaging.* Images were taken on an OLYMPUS IX71 microscope (Olympus Deutschland GmbH, Hamburg, Germany) equipped with a 10x objective (Olympus UPLanFL N 10x/0.30na) and a motorized stage (Märzhäuser Wetzlar GmbH & Co. KG, Wetzlar, Germany), allowing for the sequential recording of multiple positions. The movement of the stage was controlled by Micro-Manager 1.4. Images of three to four different positions in one well were taken with a CCD camera (OLYMPUS XM10, resolution: $1376 \times 1032$ pixels, 8 bit grey scale) at a framerate of four frames per minute. An exposure time of ten milliseconds was set. The total measurement time was limited to four hours. The focal plane was adjusted such that polystyrene particles appeared as a bright spot surrounded by a black halo (see Fig. S1).

*Image segmentation and tracking.* The image processing and tracking was done using Matlab (R2022a, MathWorks, Natick, MA, USA). It consists of two parts: corrections for imprecise stage movements, followed by the actual image segmentation. Minor inaccuracies occurred when controlling the stage of the microscope, as the stage did not exactly

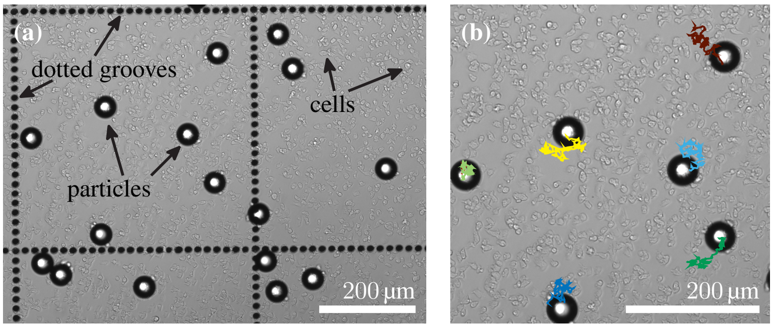


FIG. S1. Two exemplary illustrations of experimental bright-field microscopy recordings (see also Movie 1). The cargo particles with a diameter of 46 µm can be clearly identified by bright spots with a black halo. Cells with an extension of about 10 µm in the background, as exemplarily indicated by arrows, appear greyish. The small black dots in panel **(a)** that are arranged in a rectangular pattern correspond to grooves with a diameter of 5 µm that are imprinted in the polymer bottom surface of the used µ-slide for position adjustment of images that are taken at a microscope equipped with a moving stage enabling multi-position recordings (cf. Materials and Methods for details). Only those particles were tracked which move within one of these observation squares—the corresponding segment is shown in panel **(b)**, overlayed with cargo trajectories in color. The snapshot in panel **(b)** was taken 90 min after the beginning of the recording.

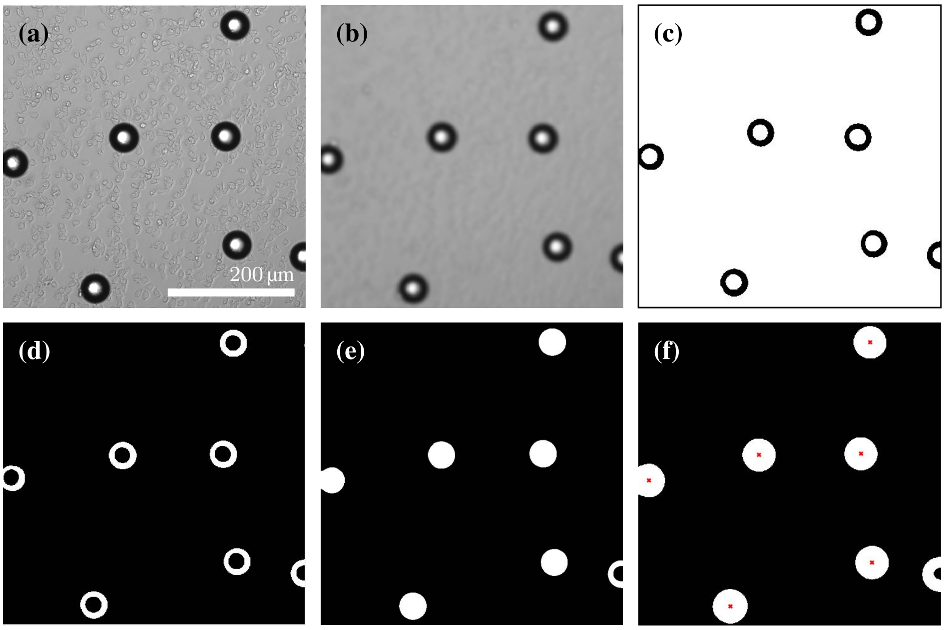


FIG. S2. Illustration of the steps for image segmentation used to track the particles within the region of interest. This sequence of steps is applied to all images separately to obtain a stack of binary masks which is afterwards used to track the positions of beads over time. The original image **(a)** is first smoothed by convolution with a Gaussian kernel **(b)** and binarized **(c)**. After inverting the resulting binary image **(d)**, holes are filled as shown in panel **(e)**. Finally, the centroid of each connected component is calculated, symbolized by red dots in panel **(f)**.

return to its original position. The grid embedded in the bottom of the µ-slide [cf. Fig. S1] enabled to detect and correct for these inaccuracies because this imprinted pattern did not move relative to the stage or µ-slide. Therefore, the location of the background pattern in each image could be compared with the location of the pattern in the first image and, thus, it was possible to calculate and subtract the spurious motion of the stage. Subsequently, a region of interest was cropped before further processing so that no part of the background grid of the µ-slide was visible to prevent tracking errors and to exclude cells from interfering with the imprinted grid (see also Fig. S1).

The individual steps of image segmentation are illustrated in Fig. S2. At first, images were smoothed (Matlab routine: *imgaussfilt* performing a convolution with a Gaussian kernel with zero mean) and binarized (Matlab routine: *imbinarize*; depending on the image quality, the option ‘adaptive’ was sometimes used). The degree of smoothing (typical value: standard deviation of $5$ to $10$ px) and the threshold for binarization (typical sensitivity level of $0.1$ for adaptive thresholding) were varied individually for each image stack. Subsequently, the binarized image was inverted (Matlab routine: *imcomplement*) and all regions that were surrounded by a closed border were filled (Matlab routine: *imfill*). To identify the beads, the area and circularity of all detected objects were determined (Matlab routine: *regionprops*) and filtered accordingly. The segmentation procedure was manually verified. Eventually, the centroid in the two-dimensional focus plane of all objects was calculated which were identified as beads before (Matlab routines: *bwconncomp* and *regionprops*).

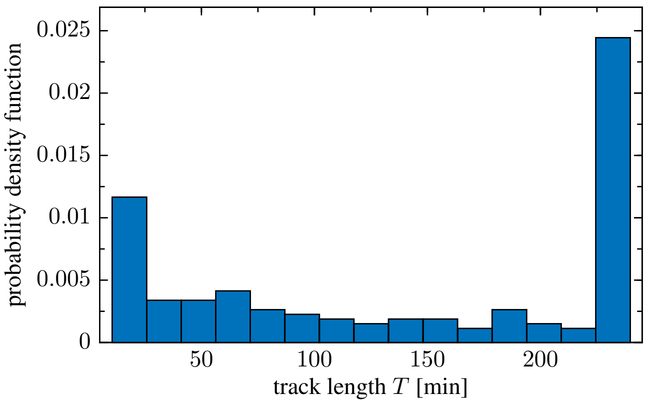


FIG. S3. Track length distribution of the recorded particle trajectories. The total recording time was four hours. Those tracks which are shorter than ten minutes were considered to be too short for a reliable statistical evaluation and were therefore discarded from the analysis. Notably, tracks with a length of four hours are most common.

The sets of centroid positions in each frame were subsequently transformed into trajectories [1]: objects with minimal distance to one another are identified with each other. In this way, the entire list of tracks was created describing the positions of beads over time in an image stack.

In total, 174 trajectories were recorded and analyzed. The distribution of track lengths is shown in Fig. S3. Notably, a significant fraction of particles could be tracked over the entire recording time of four hours. Trajectories that are shorter than ten minutes were discarded as they are considered to be too short for a reliable statistical analysis.

## STATIONARITY OF THE DYNAMICS

The mean doubling time of *D. discoideum* cells is approximately two times the duration of the experiment of 4 h [2]. Hence, the cell density grows due to cell division during the experiment. Moreover, amoeboid motility relies on the adhesion of cells to their surroundings. Since *D. discoideum* cells are adherent, they tend to stick to the particles as well. This can be seen from a comparison of Figs. S4(a,b), which shows snapshots of the system at the beginning and the end of the recording. After four hours, several cells have attached to beads, thus raising the question whether the particle dynamics is stationary. To address this question, we calculated the ensemble-average of the time-averaged mean-square displacement

$$\left\langle \overline{\delta_j^2(\tau, T)} \right\rangle = \frac{1}{T-\tau} \int_0^{T-\tau} dt \left\langle \left[\mathbf{r}_j(t+\tau) - \mathbf{r}_j(t)\right]^2 \right\rangle, \tag{S1}$$

shown in Fig. S4(c), as a function of the trajectory length $T$. It can be observed that the mean-square displacement tends to a constant for long trajectories—there is no indication that the attachment of cells to beads over time speeds up or slows down their movement significantly. Similar conclusions can be drawn from the displacement distributions shown in Figs. S4(d-e) for different time lags $\tau$: we split the trajectories in the data set into four subsets according to the corresponding measurement hours and calculated histograms of displacement distributions for each of them separately.

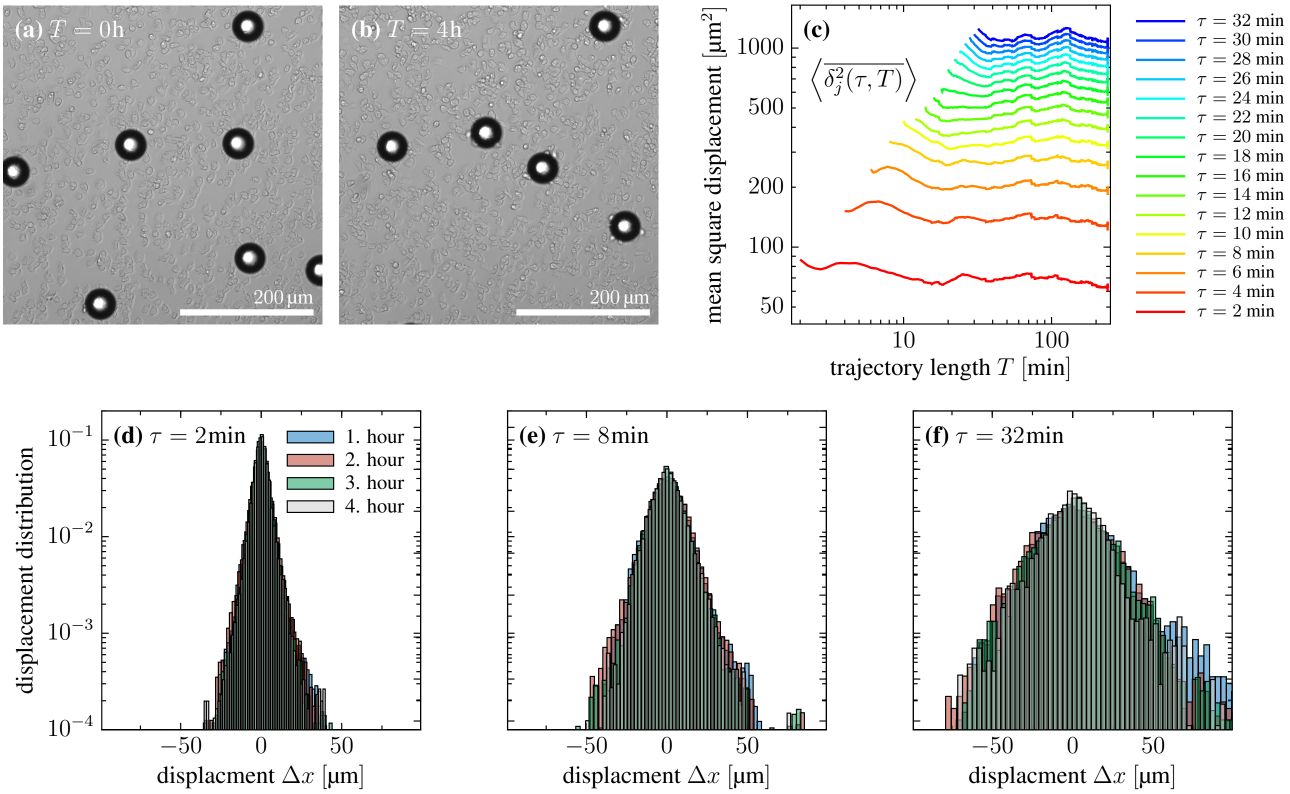


FIG. S4. The figure addresses the stationarity of the particle dynamics. In panel **(a)**, a snapshot of the system at the beginning of the recording is shown; panel **(b)** shows the same region of interest after four hours. As *D. discoideum* cells are adherent, they tend to stick to the microparticles as shown in panel **(b)**: several cells are glued to the surface of beads in the end of the recording time. Panel **(c)** shows the ensemble average of time-averaged MSDs as a function of the trajectory length $T$. It becomes constant in the limit of long trajectories, thus revealing that there is no systematic growth or decay of the MSD as a function of measurement time. Panels **(d-f)** show displacement distributions for different lag-times, however, split by hour: the histogram of all displacements from the first measurement hour are overlayed with the corresponding histograms of subsequent hours. A systematic trend is not visible. Accordingly, the dynamics of particles on cell monolayers can be considered stationary even though microscopic details, such as the global cell density and number of cells attached to a cargo particle, change over time.

The overlay does not show a significant, systematic trend. Therefore, we conclude that the stationarity of the particle dynamics driven by cells is a well-founded assumption backed up by data.

## DISPLACEMENT AUTO-CORRELATION FUNCTION FOR NORMAL BROWNIAN MOTION

In the main text, we argued that microparticles effectively perform Brownian motion for large lag times, based on the experimental observations that (i) the mean-squared displacement scales linearly in time and (ii) the displacement auto-correlation function (DACF) possesses a triangular shape. In this appendix, we derive the DACF for normal Brownian motion, described by the Langevin dynamics

$$\dot{\mathbf{r}}_j(t) = \sqrt{2D_j}\,\boldsymbol{\xi}_j(t) \tag{S2}$$

with independent Gaussian white noise processes $\boldsymbol{\xi}_j(t)$ with zero mean, $\langle \boldsymbol{\xi}_j(t) \rangle$, and temporal $\delta$-correlations: $\langle \xi_{i,\mu}(t)\xi_{j,\nu}(t') \rangle = \delta_{ij}\delta_{\mu\nu}\delta(t-t')$. The spatial particle displacement in a finite time interval $\tau$ is defined by

$$\Delta\mathbf{r}_j(t,\tau) = \mathbf{r}_j(t+\tau) - \mathbf{r}_j(t) = \sqrt{2D_j}\int_t^{t+\tau} ds\,\boldsymbol{\xi}_j(s). \tag{S3}$$

Using the formal definition of the DACF, cf. Eq. (2) in the main text, one obtains the formal expression

$$C_\tau^{(j)}(\Delta) = \frac{2D_j}{T-\Delta-\tau}\int_0^{T-\Delta-\tau} dt\left[\int_{t+\Delta}^{t+\Delta+\tau} ds \int_t^{t+\tau} ds'\,\boldsymbol{\xi}_j(s)\cdot\boldsymbol{\xi}_j(s')\right]. \tag{S4}$$

The DACF, defined via time-averaging, is again a random variable. Averaging over many realizations of the noise yields the expectation value

$$\left\langle C_\tau^{(j)}(\Delta)\right\rangle = \frac{2D_j}{T-\Delta-\tau}\int_0^{T-\Delta-\tau} dt\left[\int_{t+\Delta}^{t+\Delta+\tau} ds \int_t^{t+\tau} ds'\,\left\langle\boldsymbol{\xi}_j(s)\cdot\boldsymbol{\xi}_j(s')\right\rangle\right] \tag{S5a}$$

$$= \frac{2D_j}{T-\Delta-\tau}\int_0^{T-\Delta-\tau} dt\left[\int_{t+\Delta}^{t+\Delta+\tau} ds \int_t^{t+\tau} ds'\,2\delta(s-s')\right] \tag{S5b}$$

$$= \frac{4D_j}{T-\Delta-\tau}\int_0^{T-\Delta-\tau} dt\left[\int_{\Delta}^{\Delta+\tau} ds \int_0^{\tau} ds'\,\delta(s-s')\right] \tag{S5c}$$

$$= 4D_j\int_{\Delta}^{\Delta+\tau} ds \int_0^{\tau} ds'\,\delta(s-s') \tag{S5d}$$

$$= 4D_j\begin{cases} 0, & \Delta \geq \tau, \\ \int_\Delta^\tau ds'\,1, & 0 \leq \Delta < \tau, \\ \int_0^{\tau+\Delta} ds'\,1, & 0 > \Delta > -\tau, \\ 0, & \Delta \leq -\tau. \end{cases} \tag{S5e}$$

$$= 4D_j\begin{cases} \tau - |\Delta|, & 0 \leq |\Delta| < \tau, \\ 0, & |\Delta| \geq \tau. \end{cases} \tag{S5f}$$

For $\Delta = 0$, the linear scaling of the mean-square displacement $\langle C_\tau^{(j)}(0)\rangle = 4D_j\tau$ is recovered. Accordingly, the renormalized DACF is expected to decay linearly:

$$\frac{\langle C_\tau^{(j)}(\Delta)\rangle}{\langle C_\tau^{(j)}(0)\rangle} = \begin{cases} 1 - |\Delta|/\tau, & 0 \leq |\Delta| < \tau, \\ 0, & \text{otherwise.} \end{cases} \tag{S6}$$

In the calculation above, $\tau > 0$ is implied.

Since the correlation time of spatial displacements is finite and the increments of Brownian motion depend on time differences only (stationarity), averages over realizations of the noise $\boldsymbol{\xi}_j(t)$ and temporal averages are identical for sufficiently long trajectories:

$$\lim_{T\to\infty}\left[\frac{C_\tau^{(j)}(\Delta)}{C_\tau^{(j)}(0)}\right] = \begin{cases} 1 - |\Delta|/\tau, & 0 \leq |\Delta| < \tau, \\ 0, & \text{otherwise.} \end{cases} \tag{S7}$$

## UNIVERSAL ASYMPTOTICS OF ENSEMBLE-AVERAGED DISPLACEMENT DISTRIBUTIONS FOR HETEROGENEOUS BROWNIAN MOTION

This appendix section is concerned with the robustness of the ensemble-averaged displacement distribution with respect to the choice of the heterogeneity model $P(D)$ [Eq. (3) in the main text]. The exponential envelope of the ensemble-averaged displacement distribution, reminiscent of a Laplace PDF, is of a certain universal character as shown in the following. Given the Gaussian displacement PDF for Brownian motion

$$\rho(x|D) = \frac{1}{\sqrt{4\pi D\tau}} \exp\left[-\frac{x^2}{4D\tau}\right] \tag{S8}$$

and the heterogeneity model $P(D)$, the ensemble-averaged displacement PDF can be derived via

$$\langle\rho(x)\rangle = \int_0^\infty dD\, \rho(x|D)P(D). \tag{S9}$$

For the tails of the displacement PDF, only the behavior for large $D$ of the distribution $P(D)$ matters. As long as the distribution $P(D)$ decays exponentially,

$$P(D) \simeq f(D) \exp\left(-\frac{D}{D^*}\right) \tag{S10}$$

to leading order (the dependence $f(D)$ stands for subleading corrections), the displacement PDF will have the asymptotics

$$\langle\rho(x)\rangle \simeq \sqrt{\frac{D^*}{4\tau}} f\left(|x|\sqrt{\frac{D^*}{4\tau}}\right) \exp\left(-\frac{|x|}{\sqrt{\tau D^*}}\right), \tag{S11}$$

thus resembling the shape of a Laplace PDF.

To see that this statement holds, one starts from Eq. (S9):

$$\langle\rho(x)\rangle = \frac{1}{\sqrt{4\pi\tau}} \int_0^\infty dD\, \frac{f(D)}{\sqrt{D}} \exp\left[-\frac{x^2}{4D\tau} - \frac{D}{D^*}\right]. \tag{S12}$$

Introducing the new integration variable $\xi = D/|x|$ allows to rewrite as follows:

$$\langle\rho(x)\rangle = \sqrt{\frac{|x|}{4\pi\tau}} \int_0^\infty d\xi\, \frac{f(\xi|x|)}{\sqrt{\xi}} \exp\left[-|x|g(\xi)\right] \tag{S13}$$

with the $x$-independent function

$$g(\xi) = \frac{1}{4\tau\xi} + \frac{\xi}{D^*}. \tag{S14}$$

For large $|x|$, the integrand in Eq. (S13) is only non-negligible at the minima of $g(\xi)$. Expanding $g(\xi)$ in a Taylor series around the minimum of $g(\xi)$ at $\xi_0 = \sqrt{D^*/(4\tau)}$,

$$g(\xi) \simeq \frac{1}{\sqrt{\tau D^*}}\left[1 + \frac{2\tau}{D^*}(\xi-\xi_0)^2\right], \tag{S15}$$

yields

$$\langle\rho(x)\rangle \simeq \sqrt{\frac{|x|}{4\pi\tau}} \exp\left[-\frac{|x|}{\sqrt{\tau D^*}}\right] \int_0^\infty d\xi\, \frac{f(\xi|x|)}{\sqrt{\xi}} \exp\left[-\frac{|x|}{\sqrt{\tau D^*}}\frac{2\tau}{D^*}(\xi-\xi_0)^2\right]. \tag{S16}$$

This intermediate result already reveals the exponential envelope of the ensemble-averaged displacement PDF. Subleading order terms are derived from the remaining integral (of Gaussian type). For large $|x|$, it is dominated by values $\xi \approx \xi_0$; hence, the integration

$$\int_0^\infty d\xi\, \frac{f(\xi|x|)}{\sqrt{\xi}} \exp\left[-\frac{|x|}{\sqrt{\tau D^*}}\frac{2\tau}{D^*}(\xi-\xi_0)^2\right] = \sqrt{\xi_0}\int_0^\infty dz\, \frac{f(\xi_0|x|z)}{\sqrt{z}} \exp\left[-\frac{|x|}{\sqrt{\tau D^*}}\frac{(z-1)^2}{2}\right] \tag{S17a}$$

$$\approx \sqrt{2\pi\xi_0}\, f(\xi_0|x|)\sqrt{\frac{\sqrt{\tau D^*}}{|x|}}. \tag{S17b}$$

eventually yields Eq. (S11).

[1] J. C. Crocker and D. G. Grier, Methods of digital video microscopy for colloidal studies, J. Colloid Interface Sci. **179**, 298 (1996).
[2] J. Ashworth and D. Watts, Metabolism of the cellular slime mould *Dictyostelium discoideum* grown in axenic culture, Biochem. J. **119**, 175 (1970).
